# Supplementary material for: Enhancing Text Generation with Cooperative Training
Source: arXiv:2303.09075 source file (2023-09-23)
Supplement: Supplementary file 1 [file 6-Appendix.tex]

\section{Model Details}
\label{model training}
The 5.0B Transformer-XL is pre-trained on 32 A100s with 40G memory for 45 days, the batch size is set to 32*8=256. After running 445k steps, the final validation loss reduces to about 2.4. The 2.7B OPT is incrementally trained on the basis of the open-source model.

\begin{table}
\small
\centering
\setlength\tabcolsep{2pt} % 列间距
\caption{Statistics of Experimental Datasets}
\label{dataset}
\begin{tabular}{cccccc}
\toprule
 &  & AFQMC & CHIP-STS & QQP-ZH & MRPC \\ \midrule
\multirow{2}{*}{Zero-Shot} & \begin{tabular}[c]{@{}c@{}}domain-related\\ corpus\end{tabular} & 68668 & 32000 & 10800 & 8,152 \\
 & test dataset & 4316 & 4000 & 3600 & 1725 \\ \midrule
\multirow{2}{*}{Fine-Tune} & training dataset & 34334 & 16000 & 5400 & 4076 \\ 
 & test dataset & 4316 & 4000 & 3600 & 1725 \\ \bottomrule
\end{tabular}
\end{table}
 
During the pre-training of the generator model, we utilize the memory-cache mechanism of Transformer-XL and design a special attention mask to concatenate the multiple input sentences into one sample, to reduce the number of the padding token in a batch and therefore increase the number of effective tokens. To make the generation more robust, we add noise to the original sentences by randomly replacing or discarding tokens with a 5\% probability. In addition, the prompts that we use for Chinese generation and English generation are as follows,

\begin{itemize}
\item Chinese prompt: \begin{CJK}{UTF8}{gbsn} “$s^a$”的相似句是“$s^b$” \end{CJK} (en: A similar sentence to ``$s^a$" is ``$s^b$".)
\item English prompt: ``$s^a$" is similar to ``$s^b$"
\end{itemize}

When training the discriminator, following the usage of special tokens in BERT \cite{DBLP:conf/naacl/DevlinCLT19}, we use $[SEP]$ to concatenate two sentences and take the embedding at the $[CLS]$ position to represent the whole sentence to predict the label. Moreover, we utilize the mask method in BERT to randomly mask 15\% of the input tokens.

\section{Dataset Details}
\label{dataset setting}
The statistics of the experimental datasets are reported in Table~\ref{dataset}.

Other Chinese datasets (LCQMC \cite{liu-etal-2018-lcqmc}, OPPO, PAWS-X-zh \cite{yang-etal-2019-paws}, BQ \cite{chen-etal-2018-bq}, CCKS, Chinese-STS-B \cite{wang-etal-2018-glue}) and English datasets (QQP \cite{wang-etal-2018-glue}, STS-B \cite{wang-etal-2018-glue}, PAWS-X-en \cite{yang-etal-2019-paws}) are collected and used as the corpus of similar sentence pairs for pre-training the generator. 

The QQP-ZH dataset contains 9000 pieces of data randomly selected and translated from the English QQP dataset, which is then divided into training set and test set in a ratio of 3:2.

\section{Parameter Details}
\label{parameters}
The training parameters of zero-shot are shown in Table~\ref{zero-shot-parm}. The three thresholds are used to select positive and negative examples for training the discriminator and positive examples for training the generator, respectively. We adopt cosine annealing learning rate decay strategy during training.

\begin{table}
\small
\centering
\setlength\tabcolsep{2pt} % 列间距
\caption{Parameter Settings of Zero-Shot.}
\label{zero-shot-parm}
\begin{tabular}{l|cccc}
\toprule
 & AFQMC & CHIP-STS & QQP-ZH & MRPC \\ \midrule
\begin{tabular}[l]{@{}r@{}}Max Threshold\\ \textit{-negative}\end{tabular} & 0.8 & 0.9 & 0.95 & 0.95 \\ 
\begin{tabular}[l]{@{}r@{}}Min Threshold\\ \textit{-negative}\end{tabular} & 0.6 & 0.7 & 0.8 & 0.8 \\ 
\begin{tabular}[l]{@{}r@{}}Max Threshold\\ \textit{-positive}\end{tabular} & 0.8 & 0.9 & 0.95 & 0.95 \\ 
\begin{tabular}[l]{@{}r@{}}Min Threshold\\ \textit{-positive}\end{tabular} & 0.6 & 0.7 & 0.8 & 0.8 \\ 
\begin{tabular}[l]{@{}r@{}}Max Threshold\\ \textit{-generator}\end{tabular} & 0.6 & 0.9 & 0.95 & 0.95 \\ 
\begin{tabular}[l]{@{}r@{}}Min Threshold\\ \textit{-generator}\end{tabular} & 0.6 & 0.7 & 0.8 & 0.8 \\ 
Threshold Increase & 0.07 & 0.1 & 0.05 & 0.05 \\
Sentence Num & 6000 & 6000 & 3000 & 4000 \\ 
Learning Rate & \multicolumn{4}{c}{2e-5} \\ 
Warm Up Steps & \multicolumn{4}{c}{40} \\ 
Early Stopping & \multicolumn{4}{c}{1} \\ 
\begin{tabular}[l]{@{}r@{}}$\mathcal{G}$ Batch Size\\ \textit{-training}\end{tabular} & \multicolumn{3}{c}{2(concat 30 samples)} & 24 \\ 
\begin{tabular}[l]{@{}r@{}}$\mathcal{G}$ Batch Size\\ \textit{-predicting}\end{tabular} & \multicolumn{3}{c}{512} & 100 \\ 
\begin{tabular}[l]{@{}r@{}}$\mathcal{D}$ Batch Size\\ \textit{-training}\end{tabular} & \multicolumn{3}{c}{64} & 32 \\ 
\begin{tabular}[l]{@{}r@{}}$\mathcal{D}$ Batch Size\\ \textit{-predicting}\end{tabular} & \multicolumn{3}{c}{384} & 96 \\ \bottomrule
\end{tabular}
\end{table}

The training parameters of fine-tuning are shown in Table~\ref{fine-tune-parm}.

\begin{table}
\small
\centering
\setlength\tabcolsep{2pt} % 列间距
\caption{Parameter Settings of Fine-Tune.}
\label{fine-tune-parm}
\begin{tabular}{l|cccc}
\toprule
 & AFQMC & CHIP-STS & QQP-ZH & MRPC \\\midrule
\begin{tabular}[l]{@{}r@{}}Max Threshold\\ \textit{-negative}\end{tabular} & 0.98 & 0.98 & 0.84 & 0.8 \\ 
\begin{tabular}[l]{@{}r@{}}Min Threshold\\ \textit{-negative}\end{tabular} & 0.9 & 0.7 & 0.6 & 0.6 \\ 
\begin{tabular}[l]{@{}r@{}}Max Threshold\\ \textit{-positive}\end{tabular} & 0.98 & 0.98 & 0.98 & 0.8 \\
\begin{tabular}[l]{@{}r@{}}Min Threshold\\ \textit{-positive}\end{tabular} & 0.9 & 0.7 & 0.9 & 0.6 \\ 
\begin{tabular}[l]{@{}r@{}}Max Threshold\\ \textit{-generator}\end{tabular} & 0.98 & 0.98 & 0.98 & 0.8 \\ 
\begin{tabular}[l]{@{}r@{}}Min Threshold\\ \textit{-generator}\end{tabular} & 0.9 & 0.7 & 0.9 & 0.6 \\ 
Threshold Increase & 0.07 & 0.07 & 0.07 & 0.2 \\
Sentence Num & 6000 & 6000 & 3000 & 3000 \\
Learning Rate & \multicolumn{4}{c}{5e-6} \\
Warm Up Steps & \multicolumn{4}{c}{40} \\
Early Stopping & \multicolumn{4}{c}{1} \\
\begin{tabular}[c]{@{}r@{}}$\mathcal{G}$ Batch Size\\\textit{ -training}\end{tabular} & \multicolumn{3}{c}{2(concat 30 samples)} & 24 \\
\begin{tabular}[l]{@{}r@{}}$\mathcal{G}$ Batch Size\\\textit{ -predicting}\end{tabular} & \multicolumn{3}{c}{512} & 100 \\
\begin{tabular}[l]{@{}r@{}}$\mathcal{D}$ Batch Size\\ \textit{-training}\end{tabular} & 32 & 64 & 32 & 32 \\ 
\begin{tabular}[l]{@{}r@{}}$\mathcal{D}$ Batch Size\\ \textit{-predicting}\end{tabular} & 256 & 384 & 256 & 96 \\ \bottomrule
\end{tabular}
\end{table}

\section{The Figure of Different Threshold Functions}
\label{thre_figure}

\begin{figure*}[ht] %htbp
\begin{center}
\includegraphics[width=1.0\textwidth]{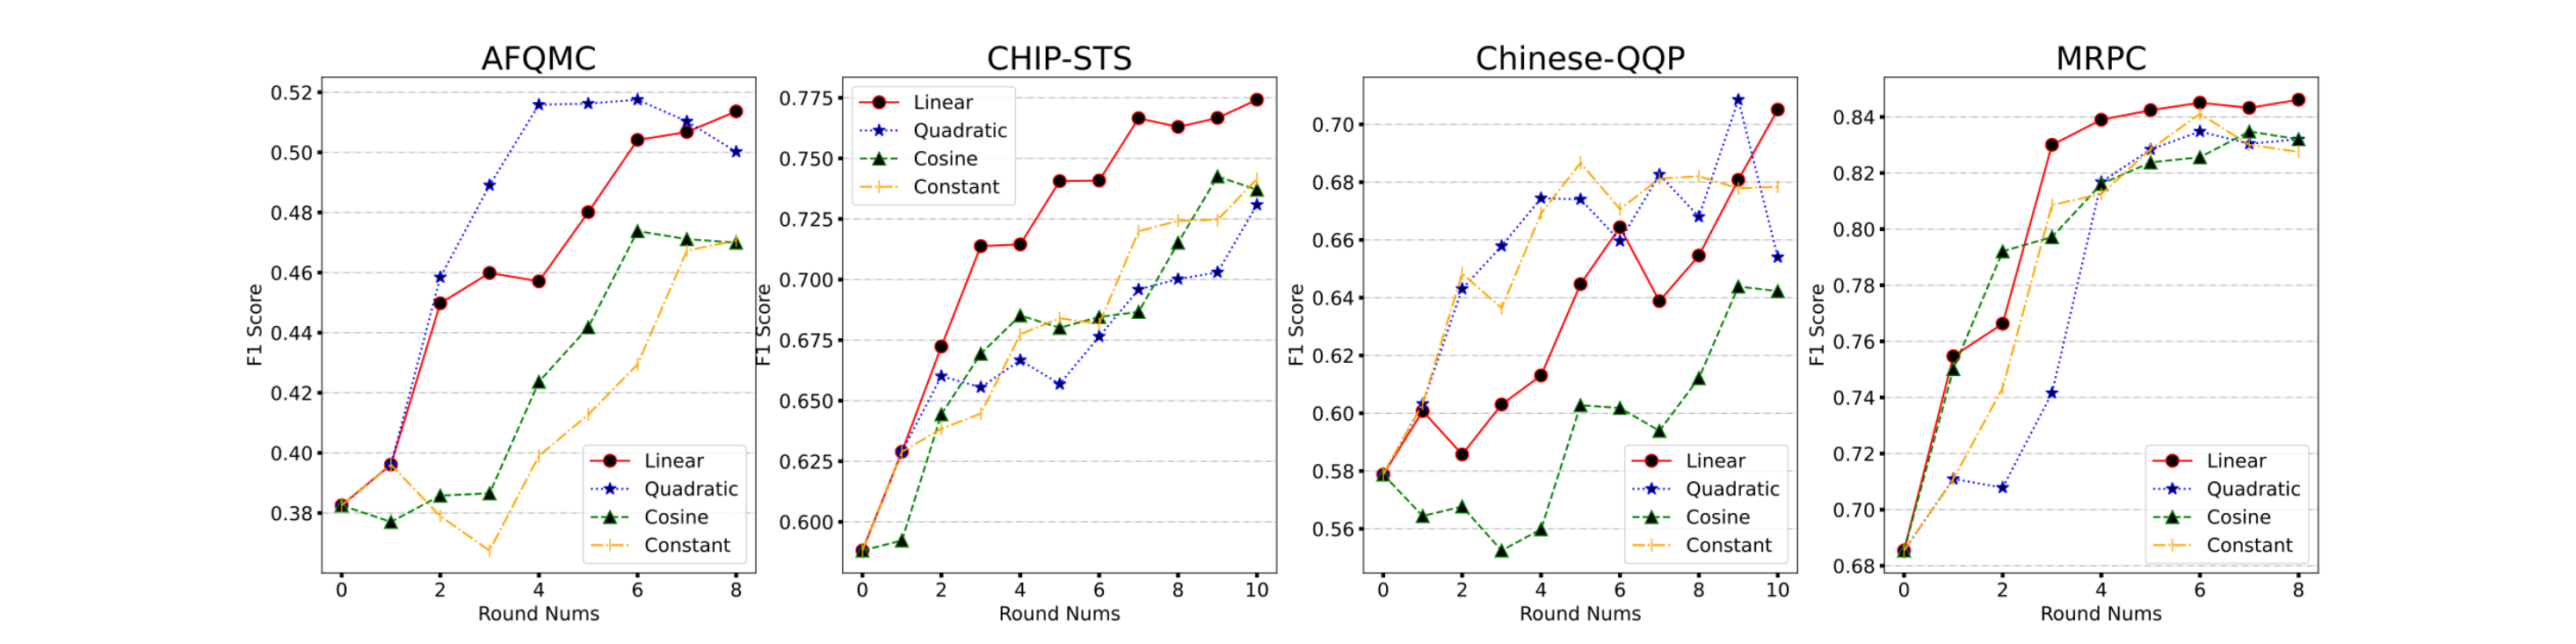}
\end{center}
\caption{Results of contrast experiments on Cosine(green), Constant(orange), Quadratic(blue) and Linear(red) function in Zero-Shot Setting.} 
\label{filter_fig}
\end{figure*}

\begin{table*}[htbp]
\caption{Generated Samples in English}
\label{samples_en}
\centering
\begin{tabular}{c}
\hline
MRPC(News) \\ \hline
\begin{tabular}[c]{@{}c@{}}\textit{origin:} Hong Kong was flat, Australia, Singapore and South Korea lost 0.2-0.4 percent.\\ \textit{first round:} the market is flat, the US is flat, Europe is flat, Japan is flat, \\ ... Malaysia is flat, Philippines is flat, Vietnam is flat, Singapore is\\ \textit{last round:} Hong Kong was unchanged, Australia, Singapore and South Korea \\ were down 0.2-0.4 percent.\end{tabular} \\ \hline
\begin{tabular}[c]{@{}c@{}}\textit{origin:} Ballmer has been vocal in the past warning that Linux is a threat to Microsoft.\\ \textit{first round:} Microsoft is a threat to Linux.\\ \textit{last round:} Ballmer has been vocal in the past about the threat Linux poses to Microsoft.\end{tabular} \\ \hline
\begin{tabular}[c]{@{}c@{}}\textit{origin:} Last year, Congress passed similar, though less expensive, buyout\\ legislation for peanut farmers, ending that Depression-era program.\\ \textit{first round:} The government is going to buy out your farm and give you a check\\ for \$1,000,000.00. You can't refuse.\\ \textit{last round:} Congress passed a similar bill last year to end a Depression-era\\ program for peanut farmers, ending that program.\end{tabular} \\ \hline
\begin{tabular}[c]{@{}c@{}}\textit{origin:} Licensing revenue slid 21 percent, however, to \$107.6 million.\\ \textit{first round:} The company's net income fell to \$1.1 million, or 2 cents per share,\\ in the quarter ended Sept. 30, from \$1.3 million, or 3 cents per share, a year earlier.\\ \textit{last round:} Licensing revenue fell 21 percent to \$107.6 million \\ in the third quarter.\end{tabular} \\ \hline
\begin{tabular}[c]{@{}c@{}}\textit{origin:} SCO says the pricing terms for a license will not \\ be announced for weeks.\\ \textit{first round:} we're not going to tell you how much it costs to buy a car, but\\ we're going to tell you how much it costs to rent one.\\ \textit{last round:} The pricing terms for a license for the SCO software will not \\ be announced for several weeks.\end{tabular} \\ \hline
\end{tabular}
\end{table*}

Figure~\ref{filter_fig} dipicts the comparison results in each round. The linear function (red line) is significantly better than the other functions on both CHIP-STS and MRPC datasets. In the AFQMC and QQP-ZH datasets, the quadratic function (blue line) is slightly more effective than the linear function. In general, we can intuitively see that all functions show a significant increase relative to the starting point.

\section{The Table of KL Divergence}
Table~\ref{consistent} shows the values of KL divergence in the first and last rounds. Numerically, it is more evident that the distances are significantly reduced on the four datasets. 

\begin{table}
\small
\centering
\setlength\tabcolsep{8pt} % 列间距
\caption{The KL divergence in the First and Last rounds of Zero-Shot.}
\label{consistent}
\sc
\begin{tabular}{l|cc}
\toprule
 & \begin{tabular}[l]{@{}r@{}}KL Divergence\\ \textit{-first round}\end{tabular} & \begin{tabular}[l]{@{}r@{}}KL Divergence\\ \textit{-last round}\end{tabular} \\ \midrule
AFQMC & 0.29 & 0.26 \\
CHIP-STS & 0.16 & 0.08 \\
QQP-ZH & 0.18 & 0.06 \\
MRPC &0.22 & 0.02 \\ \bottomrule
\end{tabular}
\end{table}

\section{Generated Samples}
\label{generate samples}
We use nucleus sampling\cite{Holtzman2020The} (with $p = 0.9$) to generate similar sentences.
Generated examples in English are shown in Table~\ref{samples_en} and in Chinese in Table~\ref{samples_zh}.

\begin{table*}[htbp]
\caption{Generated Samples in Chinese.}
\label{samples_zh}
\small
\centering
\begin{CJK}{UTF8}{gbsn}
\begin{tabular}{lcc}
\toprule
\multirow{15}{*}{\begin{tabular}[c]{@{}c@{}}AFQMC\\ (Financial)\end{tabular}} & \begin{tabular}[c]{@{}c@{}}\textit{origin：}可以用自己的支付宝为别人的花呗还款吗\\(Can I use my Alipay to repay someone else's Huabei)\\ \textit{first round：}花呗的钱可以让其他人代还吗\\(Can someone else pay for the money from Huabei)\\ \textit{last round：}花呗能不能帮别人还\\(Can my Huabei help others repay?)\end{tabular} \\ \cmidrule{2-2} 
 & \begin{tabular}[c]{@{}c@{}}\textit{origin：}花呗怎么还欠费\\(How does Huabei pay off the arrears)\\ \textit{first round：}花呗怎么还有电费\\(Why does Huabei still have electricity bills)\\ \textit{last round：}花呗还款怎么还\\(How to pay off Huabei)\end{tabular} \\ \cmidrule{2-2} 
 & \begin{tabular}[c]{@{}c@{}}\textit{origin：}我的花呗收款二维码\\(QR code for my Huabei payment)\\ \textit{first round：}商家花呗的二维码\\(Merchant Huabei's QR code)\\ \textit{last round：}花呗收款二维码在哪里\\(Where is the QR code for Huabei payment)\end{tabular} \\ \midrule
\multirow{15}{*}{\begin{tabular}[c]{@{}c@{}}CHIP-STS\\ (Medical)\end{tabular}} & \begin{tabular}[c]{@{}c@{}}\textit{origin：}艾滋病的病因是什么\\(What is the cause of AIDS)\\ \textit{first round：}艾滋病毒是什么?\\(What is HIV?)\\ \textit{last round：}艾滋病是什么原因引起的?\\(What causes AIDS?)\end{tabular} \\ \cmidrule{2-2} 
 & \begin{tabular}[c]{@{}c@{}}\textit{origin：}高血压总是流口水是怎么回事\\(High blood pressure is always drooling what is going on)\\ \textit{first round：}高血压怎么回事\\(What about high blood pressure)\\ \textit{last round：}高血压为什么会流口水?\\(Why does high blood pressure cause drooling?)\end{tabular} \\ \cmidrule{2-2} 
 & \begin{tabular}[c]{@{}c@{}}\textit{origin：}得了糖尿病,现在越来越瘦了怎么回事\\(Why am I getting thinner and thinner now that I have diabetes)\\ \textit{first round：}糖尿病现在怎么回事?\\(What's going on with diabetes now?)\\ \textit{last round：}糖尿病患者为什么会瘦?\\(Why do people with diabetes lose weight?)\end{tabular} \\ \midrule
\multirow{15}{*}{\begin{tabular}[c]{@{}c@{}}QQP-ZH\\ (Common)\end{tabular}} & \begin{tabular}[c]{@{}c@{}}\textit{origin：}如何从此网站删除我的帐户?\\(How do I delete my account from this site?)\\ \textit{first round：}怎么删除网站\\(How to delete a website)\\ \textit{last round：}如何才能删除我的帐户?\\(How can I delete my account?)\end{tabular} \\ \cmidrule{2-2} 
 & \begin{tabular}[c]{@{}c@{}}\textit{origin：}关于电子产品的一些好书是什么?\\(What are some good books on electronics?)\\ \textit{first round：}有什么好的电子产品推荐\\(Any good electronics recommendations)\\ \textit{last round：}有哪些关于电子产品的好书?\\(What are some good books about electronics?)\end{tabular} \\ \cmidrule{2-2} 
 & \begin{tabular}[c]{@{}c@{}}\textit{origin：}为什么没有人看到无尽和无限之间的区别?\\(Why does no one see the difference between endless and infinite?)\\ \textit{first round：}为什么宇宙中没有极限的存在\\(Why is there no limit in the universe)\\ \textit{last round：}为什么没有人知道无限和有限之间的区别?\\(Why does no one know the difference between infinite and finite?)\end{tabular} \\ \bottomrule
\end{tabular}
\end{CJK}
\end{table*}
